# Supplementary material for: Blue Noise Plots
Source: arXiv:2102.04072 source file (2021-02-24)
Supplement: Supplementary file 1 [file supplemental.tex]

%The study itself was set up as follow.
%First, participants got a detailed introduction into the task, including how to interpret both, the point-based visualizations, as well as a line chart.
%If participants felt confident in the task, they continued to the study.
%To keep participants motivated during the study, we presented a progress bar above the chart area, which was colored differently depending on the answer to the last question.
%If the last question was correct, we colored the bar in green, otherwise red.

%We used a side by side presentation to prevent vertical alignment of the charts and did randomly alter the which the line charts were shown at the top or the bottom.
